# Supplementary material for: Theory for magnetic-field-driven 3D metal-insulator transitions in the quantum limit
Source: arXiv:2012.12541 source file (2021-07-28)
Supplement: Supplementary file 1 [file Supp_MIT1222.pdf]

# Supplemental Material for “Theory for 3D magnetic-field-induced metal-insulator transitions in the quantum limit”

Peng-Lu Zhao,<sup>1</sup> Hai-Zhou Lu,<sup>1,2,\*</sup> and X. C. Xie<sup>3,4,5</sup>

<sup>1</sup>*Shenzhen Institute for Quantum Science and Engineering and Department of Physics, Southern University of Science and Technology (SUSTech), Shenzhen 518055, China*

<sup>2</sup>*Shenzhen Key Laboratory of Quantum Science and Engineering, Shenzhen 518055, China*

<sup>3</sup>*International Center for Quantum Materials, School of Physics, Peking University, Beijing 100871, China*

<sup>4</sup>*CAS Center for Excellence in Topological Quantum Computation, University of Chinese Academy of Sciences, Beijing 100190, China*

<sup>5</sup>*Beijing Academy of Quantum Information Sciences, West Building 3, No. 10, Xibeiwang East Road, Haidian District, Beijing 100193, China*

(Dated: December 22, 2020)

## CONTENTS

|                                            |    |
|--------------------------------------------|----|
| SI. Free Hamiltonian                       | S1 |
| A. Hamiltonian in a uniform magnetic field | S1 |
| B. Quantum limit and Linearization         | S2 |
| SII. One-Loop corrections and RG equations | S3 |
| A. One-Loop corrections                    | S3 |
| B. Renormalization-group equations         | S6 |
| C. The value of $\gamma$                   | S7 |
| SIII. Fixed point and critical exponents   | S7 |
| A. General scaling relations               | S7 |
| B. Without disorder                        | S8 |
| C. With forward-scattering disorder        | S8 |
| D. With backscattering disorder            | S9 |
| References                                 | S9 |

## SI. FREE HAMILTONIAN

### A. Hamiltonian in a uniform magnetic field

Based on [1–3], the low-energy Hamiltonian of ZrTe<sub>5</sub> around the  $\Gamma$  point reads,

$$H = \sum_{\mathbf{k}} \Psi_{\mathbf{k}}^{\dagger} [m(\mathbf{k}) \tau_z \sigma_0 + \hbar v_x k_x \tau_x \sigma_z + \hbar v_y k_y \tau_y \sigma_0 + \hbar v_z k_z \tau_x \sigma_x] \Psi_{\mathbf{k}}, \quad (\text{S1})$$

where  $\Psi_{\mathbf{k}} = (c_{\mathbf{k},+, \uparrow}, c_{\mathbf{k},+, \downarrow}, c_{\mathbf{k},-, \uparrow}, c_{\mathbf{k},-, \downarrow})$ , and  $+, -$  label the two states of each Kramer pair at the  $\Gamma$  point, which form the pseudo orbital degrees of freedom. Here  $\tau$  and  $\sigma$  are Pauli matrices operating on the pseudo orbital and spin spaces, respectively, and  $c_{\mathbf{k}, \tau_z, \sigma_z}$  are the annihilation operators for the basis states  $|\tau_z = \pm 1, S_z = \pm \frac{1}{2}\rangle$  with wavevector  $\mathbf{k}$ .  $v_{x,y,z}$  are real parameters for the anisotropic “Fermi velocities”, and the “Dirac mass” is given by [2, 4]

$$m(\mathbf{k}) = M_0 + M_1 (v_x^2 k_x^2 + v_y^2 k_y^2) + M_z k_z^2, \quad (\text{S2})$$

where  $M_0, M_1, M_z$  are the real model parameters.

---

\* Corresponding author: luhz@sustech.edu.cn

To obtain the Landau levels, we consider a uniform magnetic field  $\mathbf{B} = B\mathbf{e}_z$  along the  $z$  direction, which corresponds to the crystallographic  $b$  axis in the experiment [2]. We employ a Landau-gauge vector potential  $\mathbf{A} = (-By, 0, 0)$  to describe the uniform magnetic field, and with this vector potential, the low-energy Hamiltonian density becomes

$$\mathcal{H}(\mathbf{k}) = m \left( k_x - \frac{eB}{\hbar} y, k_y, k_z \right) \tau_z \sigma_0 + \hbar v_x \left( k_x - \frac{eB}{\hbar} y \right) \tau_x \sigma_z + \hbar v_y k_y \tau_y \sigma_0 + \hbar v_z k_z \tau_x \sigma_x. \quad (\text{S3})$$

Therefore  $[k_x, \mathcal{H}(\mathbf{k})] = 0 = [k_z, \mathcal{H}(\mathbf{k})]$ , which means that the wave vector  $k_{y,z}$  are still good quantum numbers. The eigen states can be generally written as

$$\Psi = \Psi(y) e^{i(k_x x + k_z z)/\hbar}, \quad (\text{S4})$$

where  $\Psi(y)$  is a  $4 \times 1$  matrix. To solve  $\Psi(y)$ , we consider  $v_x v_y B > 0$  [1, 4] and define the ladder operators

$$a = \frac{\ell_B}{\sqrt{2}v_\perp} \left[ v_x \left( k_x - \frac{eB}{\hbar} y \right) - v_y \partial_y \right], \\ a^\dagger = \frac{\ell_B}{\sqrt{2}v_\perp} \left[ v_x \left( k_x - \frac{eB}{\hbar} y \right) + v_y \partial_y \right], \quad (\text{S5})$$

where  $v_\perp = \sqrt{v_x v_y}$  and  $\ell_B = \sqrt{\hbar/(eB)}$  is the magnetic length. One can check that  $[a, a^\dagger] = 1$ , and the eigenstates for the occupation number operator of these ladder operators can be obtained by solving  $c^\dagger c |n\rangle = n |n\rangle$ . With the eigenstates  $\{|n\rangle\}$ ,  $\Psi(y)$  is proportional to the wave function  $(|n-1\rangle, |n\rangle, |n\rangle, |n-1\rangle)^T$ , where  $c|n\rangle = \sqrt{n}|n-1\rangle$  and  $c^\dagger|n-1\rangle = \sqrt{n}|n\rangle$ . In the basis, the original Hamiltonian density Eq. (S3) takes the form

$$\mathcal{H}_n(\mathbf{k}) = \begin{pmatrix} m_-(k_z) & 0 & \frac{\sqrt{2}v_\perp \hbar}{\ell_B} \sqrt{n} & v_z \hbar k_z \\ 0 & m_+(k_z) & v_z \hbar k_z & -\frac{\sqrt{2}v_\perp \hbar}{\ell_B} \sqrt{n} \\ \frac{\sqrt{2}v_\perp \hbar}{\ell_B} \sqrt{n} & v_z \hbar k_z & -m_+(k_z) & 0 \\ v_z \hbar k_z & -\frac{\sqrt{2}v_\perp \hbar}{\ell_B} \sqrt{n} & 0 & -m_-(k_z) \end{pmatrix}, \quad (\text{S6})$$

where

$$m_\pm(k_z) = M_0 + \frac{M_\perp}{\ell_B^2} (2n \pm 1) + M_z k_z^2, \quad (\text{S7})$$

$M_\perp = M_1 v_\perp^2$ , and  $n \geq 0$  is the Landau level index.

## B. Quantum limit and Linearization

According to [2], the metal-insulators happens at a critical magnetic field of  $B_c = 6.71\text{T}$ , which is much larger than the magnetic field  $B_Q = 1.3\text{T}$  when entering the quantum limit. Therefore, the metal-insulators happens in the deep quantum limit, only the 0<sup>th</sup> Landau level is occupied by the electrons, so we only focus on the  $n = 0$  case, the wave function is proportional to  $(0, |0\rangle, |0\rangle, 0)^T$ , the single-particle Hamiltonian density becomes

$$\mathcal{H}_{n=0}(\mathbf{k}) = \begin{pmatrix} m_+(k_z) & v_z \hbar k_z \\ v_z \hbar k_z & -m_+(k_z) \end{pmatrix} = m_+(k_z) \sigma_z + \hbar v_z k_z \sigma_x, \quad (\text{S8})$$

Its energy eigenvalues are

$$E_{0\pm}(k_z) = \pm \sqrt{(\hbar v_z k_z)^2 + m_+^2(k_z)}. \quad (\text{S9})$$

When the Fermi energy  $E_F$  crosses one of the above energy bands at the two Fermi wave vectors  $\pm k_F \mathbf{e}_z$ , we need to linearize the energy dispersion around two Fermi wave vectors  $\pm k_F \mathbf{e}_z$  and obtain the interaction-free Hamiltonian which dominates the related physics. Suppose we have a positive Fermi energy  $E_F$  which crosses the  $E_{0+}(k_z)$  band, by using of the standard linearization scheme [5, 6], the energy dispersion  $E_{0+}(k_z)$  can be written as

$$E_{0+}(k_z) = \begin{cases} v_F \hbar k_z, & \text{for } k_z \text{ near } k_F; \\ -v_F \hbar k_z, & \text{for } k_z \text{ near } -k_F, \end{cases} \quad (\text{S10})$$

where the effective Fermi velocity is

$$v_F = \left| \frac{1}{\hbar} \frac{dE_{0+}}{dk_z} \right|_{k_z=k_F} = \left| \frac{(\hbar v_z)^2 k_F + 2m_+(k_F) M_z k_F}{\hbar \sqrt{(\hbar v_z k_F)^2 + m_+^2(k_F)}} \right|. \quad (\text{S11})$$

In the basis of  $\psi(\mathbf{k}) = (\psi_-(\mathbf{k}), \psi_+(\mathbf{k}))^T$ , the effective free Hamiltonian for ZrTe<sub>5</sub> in the quantum limit is given by

$$H_0 = \sum_{\mathbf{k}} \psi^\dagger(\mathbf{k}) v_F \hbar k_z \sigma_z \psi(\mathbf{k}), \quad (\text{S12})$$

where  $\psi_\pm^\dagger(\mathbf{k})$  and  $\psi_\pm(\mathbf{k})$  are the creation and annihilation operators in the vicinity of  $\mp k_F$ , and the wave vector  $\mathbf{k}$  in  $\psi_\pm^\dagger(\mathbf{k})$  is defined to be relative to the Fermi wave vector  $\pm k_F \mathbf{e}_z$ .

### SII. ONE-LOOP CORRECTIONS AND RG EQUATIONS

#### A. One-Loop corrections

The total action takes the form

$$\begin{aligned} S &= S_0 + S_b + S_p + S_e + S_d, \\ S_0 &= \int d^3\mathbf{k} d\omega \psi^\dagger (-i\omega + v_F k_z \sigma_z) \psi, \\ S_b &= \int d^3\mathbf{k} d\omega \left[ \phi^* (\omega^2 + v_b^2 \mathbf{k}^2 + r) \phi + h |\phi|^4 \right], \\ S_p &= \int d^3x d\tau g \left( \phi \psi_+^\dagger \psi_- + \phi^* \psi_-^\dagger \psi_+ \right) = \int d^d x d\tau g \left( \phi \psi^\dagger \sigma^- \psi + h.c. \right), \\ S_e &= u \int d^3x d\tau \psi_+^\dagger \psi_+ \psi_-^\dagger \psi_- = u \int d^d x d\tau (\psi^\dagger \Gamma^- \psi) (\psi^\dagger \Gamma^+ \psi), \\ S_d &= - \sum_{i=f,b} \frac{\Delta_i}{2} \int d^3x d\tau d\tau' (\psi^\dagger \Gamma_i \psi)_\tau (\psi^\dagger \Gamma_i \psi)_{\tau'}, \end{aligned} \quad (\text{S13})$$

where  $\sigma^\pm = (\sigma_x \pm i\sigma_y)/2$ ,  $\Gamma_\pm = (\sigma_0 \pm \sigma_z)/2$ ,  $v_b$  represents the phonon speed, and  $r = 0$  at the quantum critical point. We have ignored the fluctuation of the order parameters, which originates from the interaction between phonons and usually takes a form as  $h |\phi|^4$ . Although this fluctuation is strong at the quantum critical point, it gives second-order contributions to the values of critical exponents, and hence this term can be neglected in our analysis. We have included the forward-scattering disorder and  $2k_F$ -scattering disorder in  $S_d$ , but we remind that only one type of disorder is considered for our RG calculation below, we do not consider the coexistence of different types of disorder.

The clean, noninteracting propagators for fermions and bosons are given by

$$D_0(\omega, \mathbf{k}) = \frac{1}{\omega^2 + v_b^2 \mathbf{k}^2}, \quad (\text{S14})$$

$$G_0(\omega, \mathbf{k}) = \frac{i\omega + v_F k_z \sigma_z}{\omega^2 + v_F^2 k_z^2}. \quad (\text{S15})$$

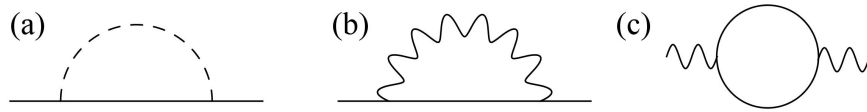

FIG. S1. (a),(b) One-loop self-energy corrections to fermions. (c) One-loop self-energy correction to bosons. The solid, dashed, and wavy lines stand for the fermion, disorder, and boson, respectively

**Self-energy corrections:** We show the self-energy corrections to fermions and bosons in Fig. S1. Figure S1(a)

accounts for the fermionic self-energy correction due to electron-phonon interactions, which is given by

$$\begin{aligned}\Sigma_a(\mathbf{q}, \Omega) &= -g^2 \int \frac{d^3\mathbf{k}}{(2\pi)^3} \int \frac{d\omega}{2\pi} [\sigma^+ G_0(\mathbf{k}, \omega) \sigma^- + \sigma^- G_0(\mathbf{k}, \omega) \sigma^+] D_0(\mathbf{q} - \mathbf{k}, \Omega - \omega) \\ &= -\frac{g^2 \ell}{4\pi^2 \ell_B^2 v_b^3 \Lambda^2} \left[ \frac{\gamma^2}{(\gamma + 1)^2} (i\Omega) - \frac{\gamma^2 (2\gamma + 1)}{(\gamma + 1)^2} (v_F q_z \sigma_z) \right],\end{aligned}\quad (\text{S16})$$

where  $\gamma = |v_b/v_F|$ . The momentum-frequency integration is performed as

$$\int \frac{d^3\mathbf{k}}{(2\pi)^3} \int \frac{d\omega}{2\pi} = \int \frac{dk_z}{2\pi} \int_{-\infty}^{+\infty} \frac{d\omega}{2\pi} \int \frac{dk_x dk_y}{(2\pi)^2} = \frac{1}{2\pi \ell_B^2} \left( \int_{-\Lambda}^{-\Lambda e^{-\ell}} + \int_{\Lambda e^{-\ell}}^{\Lambda} \right) \frac{dk_z}{2\pi} \int_{-\infty}^{+\infty} \frac{d\omega}{2\pi}.\quad (\text{S17})$$

Figure S1(b) represents the fermions self-energy correction from disorder and gives rise to

$$\begin{aligned}\Sigma_b(i\Omega) &= -\Delta_i \int \frac{d^d\mathbf{q}}{(2\pi)^d} \Gamma_i G_0(i\Omega, \mathbf{q}) \Gamma_i \\ &= -\frac{a_i \Delta_i \ell}{2\pi^2 v_F^2 \ell_B^2 \Lambda^\epsilon} (i\Omega),\end{aligned}\quad (\text{S18})$$

where  $a_{(f,b)} = (1, 2)$ . The boson self-energy correction shown in Fig. S1(c) reads

$$\begin{aligned}\Pi(\Omega, \mathbf{p}) &= -g^2 \int \frac{d^3\mathbf{k}}{(2\pi)^3} \int \frac{d\omega}{2\pi} \text{Tr} [\sigma^- G_0(\omega, \mathbf{k}) \sigma^+ G_0(\omega + \Omega, \mathbf{k} + \mathbf{p})] \\ &= -\frac{g^2}{2\pi^2 \ell_B^2} \ln \left( \frac{-2k_F v_F + p_z v_F + i\Omega}{2v_F k_F + v_F p_z + i\Omega} \right),\end{aligned}\quad (\text{S19})$$

which leads to the Kohn anomaly [6, 7] in one or quasi-one dimensional systems.

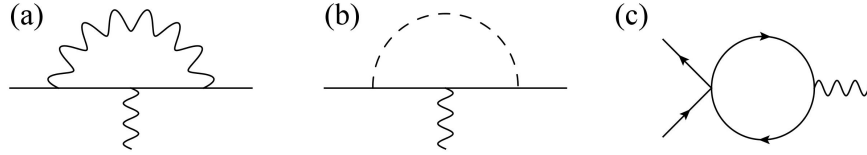

FIG. S2. One-loop corrections to the vertex of electron-phonon interactions.

**Electron-phonon coupling corrections:** All the one-loop corrections to the electron-phonon vertex are shown in Fig. S2. The contribution from Fig. S2(a) goes as

$$\begin{aligned}\delta g_a &= g^3 \int \frac{d^3\mathbf{k}}{(2\pi)^d} \int \frac{d\omega}{2\pi} [\phi \psi^\dagger (\sigma^- G_0(\mathbf{k}, \omega) \sigma^\pm G_0(\mathbf{k}, \omega) \sigma^+ + \sigma^+ G_0(\mathbf{k}, \omega) \sigma^\pm G_0(\mathbf{k}, \omega) \sigma^-) \psi + h.c.] D_0(\mathbf{k}, \omega) \\ &= 0\end{aligned}\quad (\text{S20})$$

The Fig. S2(b) stands for the corrections due to disorder and is given by

$$\begin{aligned}\delta g_b &= g \Delta_j \int \frac{d^3\mathbf{k}}{(2\pi)^d} [\phi \psi^\dagger (\Gamma_j G_0(\mathbf{k}, 0) \sigma^- G_0(\mathbf{k}, 0) \Gamma_j) \psi + h.c.] \\ &= \begin{cases} \frac{-g \Delta_f \ell}{2\pi^2 v_F^2 \ell_B^2 \Lambda} (\phi \psi^\dagger \sigma^- \psi + h.c.), & j = f; \\ \frac{-g \Delta_b \ell}{\pi^2 v_F^2 \ell_B^2 \Lambda} (i \phi \psi^\dagger \sigma^+ \psi + h.c.), & j = b. \end{cases}\end{aligned}\quad (\text{S21})$$

Note that  $(i \phi \psi^\dagger \sigma^+ \psi + h.c.)$  is not present in the original action. This term represents the  $\mathbf{q} = 0$  case for the electron-phonon interaction, which is not related to our physics ( $\mathbf{q} = \pm 2k_F \mathbf{e}_z$ ). Besides, this term has only the  $O(\Delta_{x,y})$  contribution. We will neglect this term, and hence Fig. S2(b) only gives a correction as

$$\delta g_b = -\frac{g \Delta_f \ell}{2\pi^2 v_F^2 \ell_B^2 \Lambda} (\phi \psi^\dagger \sigma^- \psi + h.c.).\quad (\text{S22})$$

The corrections due to electron-electron interaction is shown in Fig. S2(c), which takes the form

$$\begin{aligned}\delta g_c &= -gu \int \frac{d^3\mathbf{k}}{(2\pi)^d} \int \frac{d\omega}{2\pi} [\phi\psi^\dagger (\Gamma^+ G_0(\mathbf{k}, \omega) \sigma^- G_0(\mathbf{k}, \omega) \Gamma^- + \Gamma^- G_0(\mathbf{k}, \omega) \sigma^- G_0(\mathbf{k}, \omega) \Gamma^+) \psi + h.c.] \\ &= \frac{gu\ell}{4\pi^2 v_F \ell_B^2} (\phi\psi^\dagger \sigma^- \psi + h.c.).\end{aligned}\quad (\text{S23})$$

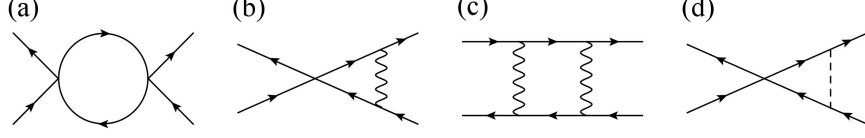

FIG. S3. One-loop corrections to the vertex of electron-phonon.

**Electron-electron vertex corrections:** All the one-loop corrections to the electron-electron vertex are shown in Fig. S3. The contribution from Fig. S3(a) goes as [8]

$$\begin{aligned}\delta u_a &= -2u^2 \int \frac{d^3\mathbf{k}}{(2\pi)^3} \int \frac{d\omega}{2\pi} [\psi^\dagger (\Gamma^- G_0(\mathbf{k}, \omega) \Gamma^-) \psi] [\psi^\dagger (\Gamma^+ G_0(\mathbf{k}, \omega) \Gamma^+) \psi] \\ &= \frac{u^2 \ell}{2\pi^2 v_F \ell_B^2} (\psi^\dagger \Gamma^- \psi) (\psi^\dagger \Gamma^+ \psi).\end{aligned}\quad (\text{S24})$$

The correction from Fig. S3(b) is given by

$$\begin{aligned}\delta u_b &= g^2 u \int \frac{d^3\mathbf{k}}{(2\pi)^3} \int \frac{d\omega}{2\pi} \{ [\psi^\dagger (\sigma_- G_0(\mathbf{k}, \omega) \Gamma^-) \psi \psi^\dagger (\Gamma^+ G_0(\mathbf{k}, \omega) \sigma_+) \psi + (\Gamma^- \leftrightarrow \Gamma^+)] + [\sigma_- \leftrightarrow \sigma_+] \} D_0(\mathbf{k}, \omega) \\ &= 0.\end{aligned}\quad (\text{S25})$$

The contribution from Fig. S3(c) can be written as

$$\begin{aligned}\delta u_c &= -\frac{g^4}{2} \int \frac{d^3\mathbf{k}}{(2\pi)^3} \int \frac{d\omega}{2\pi} \{ [\psi^\dagger (\sigma_- G_0(\mathbf{k}, \omega) \sigma_-) \psi \psi^\dagger (\sigma_+ G_0(\mathbf{k}, \omega) \sigma_+) \psi \\ &\quad + \psi^\dagger (\sigma_- G_0(\mathbf{k}, \omega) \sigma_+) \psi \psi^\dagger \sigma_- G_0(-\mathbf{k}, -\omega) \sigma_+ \psi] + h.c. \} D_0^2(\mathbf{k}, \omega) \\ &= 0.\end{aligned}\quad (\text{S26})$$

The contribution from Fig. S3(d) is given by

$$\begin{aligned}\delta u_d &= u \Delta_i \int \frac{d^3\mathbf{k}}{(2\pi)^3} \{ [(\psi^\dagger (\Gamma_i G_0(\mathbf{k}, 0) \Gamma^-) \psi) (\psi^\dagger (\Gamma^+ G_0(\mathbf{k}, 0) \Gamma_i) \psi)] + [\Gamma^- \leftrightarrow \Gamma^+] \} \\ &= \begin{cases} \frac{-u \Delta_f \ell}{\pi^2 v_F^2 \ell_B^2 \Lambda} (\psi^\dagger \Gamma^- \psi) (\psi^\dagger \Gamma^+ \psi), & i = f; \\ 0, & i = b. \end{cases}\end{aligned}\quad (\text{S27})$$

**Disorder vertex corrections:** All the one-loop corrections to the electron-electron vertex are shown in Fig. S3. The contribution from Fig. S3(a) goes as

$$\begin{aligned}\delta \Delta_i^a &= -\Delta_i^2 (\psi^\dagger \Gamma_i \psi) \psi^\dagger \int \frac{d^3\mathbf{k}}{(2\pi)^3} \Gamma_i G(\mathbf{k}, 0) \Gamma_i G(\mathbf{k}, 0) \Gamma_i \psi \\ &= \begin{cases} \frac{-\Delta_f^2 \ell}{2\pi^2 v_F^2 \ell_B^2 \Lambda} (\psi^\dagger \sigma_0 \psi) (\psi^\dagger \sigma_0 \psi), & i = f; \\ \frac{2\Delta_b^2 \ell}{2\pi^2 v_F^2 \ell_B^2 \Lambda} [\psi^\dagger (\sigma_x + \sigma_y) \psi] [\psi^\dagger (\sigma_x + \sigma_y) \psi], & i = b. \end{cases}\end{aligned}\quad (\text{S28})$$

The correction from Fig. S3(b) is given by

$$\begin{aligned}\delta \Delta_i^b &= -g^2 \Delta_i (\psi^\dagger \Gamma_i \psi) \psi^\dagger \int \frac{d^3\mathbf{k}}{(2\pi)^3} \int \frac{d\omega}{2\pi} [\sigma^+ G(\mathbf{p}, \omega) \Gamma_i G(\mathbf{p}, \omega) \sigma^- + (\sigma^- \leftrightarrow \sigma^+)] \psi D_0(\mathbf{k}, \omega) \\ &= \begin{cases} \frac{-g^2 \Delta_f \gamma^2 \ell}{4\pi^2 v_b^3 \ell_B^2 \Lambda^2 (\gamma + 1)^2} (\psi^\dagger \sigma_0 \psi) (\psi^\dagger \sigma_0 \psi), & i = f; \\ 0, & i = b. \end{cases}\end{aligned}\quad (\text{S29})$$

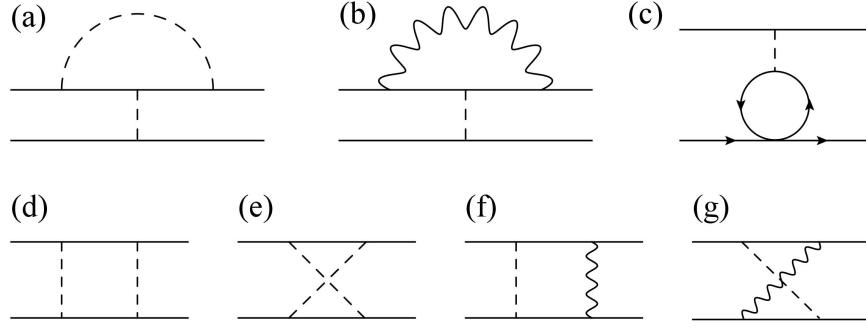

FIG. S4. One-loop corrections to the vertex of electron-phonon.

The contribution from Fig. S3(c) reads

$$\begin{aligned} \delta\Delta_i^c &= u\Delta_i (\psi^\dagger \Gamma_i \psi) \psi^\dagger \int \frac{d^3\mathbf{k}}{(2\pi)^3} \int \frac{d\omega}{2\pi} [\Gamma_+ G(\mathbf{k}, \omega) \Gamma_i G(\mathbf{k}, \omega) \Gamma_- + (\Gamma_+ \leftrightarrow \Gamma_-)] \psi \\ &= \begin{cases} 0, & i = f; \\ \frac{-u\Delta_b \ell}{4\pi^2 \ell_B^2 v_F} [\psi^\dagger (\sigma_x + \sigma_y) \psi] [\psi^\dagger (\sigma_x + \sigma_y) \psi], & i = b. \end{cases} \end{aligned} \quad (\text{S30})$$

The contribution from Fig. S3(d) and Fig. S3(e) together is given by

$$\begin{aligned} \delta\Delta_i^{d+e} &= -\Delta_i^2 \int \frac{d^3\mathbf{k}}{(2\pi)^3} \psi^\dagger [\Gamma_i G_0(\mathbf{k}, 0) \Gamma_i] \psi \psi^\dagger [\Gamma_i G_0(\mathbf{k}, 0) \Gamma_i + \Gamma_i G_0(-\mathbf{k}, 0) \Gamma_i] \psi \\ &= 0. \end{aligned} \quad (\text{S31})$$

In principle, Fig. S3(f) and Fig. S3(g) could renormalize both the electron-electron interaction and disorder vertices. However, the direct calculations show that these two diagrams do not renormalize any vertex.

## B. Renormalization-group equations

After finishing the calculations of loop corrections, one can insert all the corrections into the free action, and make the standard rescalings [9, 10], then the following renormalization-group equations can be obtained as

$$\frac{dv_F}{d\ell} = \left[ z - 1 + \frac{2g^2\gamma^3}{(\gamma+1)^2} - a_i\Delta_i \right] v_F, \quad (\text{S32})$$

$$\frac{d\Delta_f}{d\ell} = \left[ 2\Delta_f + 1 - \frac{4g^2\gamma^3}{(\gamma+1)^2} \right] \Delta_f, \quad (\text{S33})$$

$$\frac{d\Delta_b}{d\ell} = -4\Delta_b^2 + \left[ 1 + 2u - \frac{2g^2\gamma^2(2\gamma+1)}{(\gamma+1)^2} \right] \Delta_b, \quad (\text{S34})$$

$$\frac{dg^2}{d\ell} = -\frac{2(g^2)^2\gamma^2}{(\gamma+1)^2} + (2 + 2u - 2b_i\Delta_i)g^2, \quad (\text{S35})$$

$$\frac{du}{d\ell} = 2u^2 - \left( \frac{2g^2\gamma^2}{\gamma+1} + c_i\Delta_i \right) u. \quad (\text{S36})$$

where  $a_{(f,b)} = (1, 2)$ ,  $b_{(f,b)} = (2, 2)$ ,  $c_{(f,b)} = (3, 2)$ , and there is no autosum of the repeated index  $i$ . We have introduced dimensionless coupling parameters by making the following redefinitions of the couplings as

$$\frac{g^2}{4\pi^2 \ell_B^2 v_b^3 \Lambda^2} \rightarrow \beta, \quad \frac{u}{4\pi^2 v_F \ell_B^2} \rightarrow u, \quad \frac{\Delta_i}{2\pi^2 v_F^2 \ell_B^2 \Lambda} \rightarrow \Delta_i \quad (\text{S37})$$

These renormalization-group equation establish only when a single type of disorder is included, we do not consider the coexistence of any two kinds of disorder. With this consideration, these renormalization-group equations become the equations shown in the main text.

### C. The value of $\gamma$

Our renormalization-group equations are highly dependent on the parameter  $\gamma = |v_b/v_F|$ . According to Eq. (S19), the vacuum bubble diagram Fig. S1 gives rise to the Kohn anomaly [6, 7], but does not renormalize the phonon velocity  $v_b$ . Moreover, we keep  $v_F$  fixed to obtain a scale dependent dynamic exponent  $z$ . As a result,  $\gamma = |v_b/v_F|$  is a scale independent constant, and we need to determine its value by means of the model parameters. By definition

$$v_F = \left| \frac{(\hbar v_z)^2 k_F + 2m_+(k_F) M_z k_F}{\hbar \sqrt{(\hbar v_z k_F)^2 + m_+^2(k_F)}} \right|. \quad (\text{S38})$$

The Fermi wave vector of the lowest Landau band is given by [3, 11, 12]

$$k_F = \frac{2\pi^2 \hbar n}{eB}, \quad (\text{S39})$$

where  $n$  is carrier density. By using the following parameters [1–4]:  $n = n_0 = 8.87 \times 10^{16} \text{cm}^{-3}$ ,  $v_x = 9 \times 10^5 \text{m/s}$ ,  $v_y = 1.9 \times 10^5 \text{m/s}$ ,  $v_z = 0.3 \times 10^5 \text{m/s}$ ,  $M_0 = -4.7 \text{meV}$ ,  $M_\perp = 150 \text{meV} \cdot \text{nm}^2$ ,  $M_z = 0.01 M_\perp$ , we obtain a Fermi velocity as  $v_F \approx 2.9 \times 10^5 \text{m/s} \approx v_z$ . It is believed that acoustic phonons play a dominant role in the formation of CDW [3], and according to previous DFT calculation, the velocities for the acoustic phonons of  $\text{ZrTe}_5$  at the  $\Gamma$ -point along the  $a$ ,  $b$ ,  $c$  axis are 2217m/s, 494m/s, and 2185m/s, respectively [13]. As a result,  $\gamma = |v_b/v_F| \approx 1.7 \times 10^{-3}$ , which is a small quantity in our calculations.

## III. FIXED POINT AND CRITICAL EXPONENTS

### A. General scaling relations

Provided the transition is controlled by the magnetic field and happens at a critical value  $B_c$ , a divergent length is given by [14, 15]

$$\zeta \sim |B - B_c|^{-\nu_B}, \quad (\text{S40})$$

where  $\nu_B$  is the correlation length exponent defined by the magnetic field. A vanishing characteristic frequency is determined by

$$\Omega \sim \zeta^{-z} \sim |B - B_c|^{z\nu_B} \sim k_B T / \hbar, \quad (\text{S41})$$

where  $z$  is the dynamical exponent, and  $k_B$  is the Boltzmann constant. According to [15, 16], the finite-size scaling formula for resistivity reads

$$\rho(B, T) = \rho(B_c) f_B[|B - B_c| / T^{1/z\nu_B}], \quad (\text{S42})$$

where  $f_{i=B}(x)$  is a scaling function with  $f(0) = 1$ . However, the correlation length exponent is obtained by the divergent coupling strength for our renormalization-group calculation, we need to fix its connection with the magnetic field. Taking the electron-phonon coupling  $\beta$  as an example,

$$\beta = \frac{g^2}{4\pi^2 \ell_B^2 v_b^3 \Lambda^2} \sim \frac{g^2}{4\pi^2 \ell_B^2 v_b^3 k_F^2} \sim g^2 B^3, \quad (\text{S43})$$

where we have taken  $\Lambda \sim k_F$  because the momentum is defined to be relative to the Fermi wave vector  $\pm k_F \mathbf{e}_z$ . As a result,

$$\zeta \sim |\beta - \beta_c|^{-\nu_\beta} \sim |B - B_c|^{-3\nu_\beta}, \quad (\text{S44})$$

and

$$\rho(B, T) = \rho(B_c) f_\beta[|B - B_c| / T^{1/3z\nu_\beta}]. \quad (\text{S45})$$

If the correlation length exponent is obtained by divergent electron-electron interactions, the resistivity should satisfy the scaling forms,

$$\rho(B, T) = \rho(B_c) f_u[|B - B_c| / T^{1/z\nu_u}]. \quad (\text{S46})$$

For the forward-scattering disorder,

$$\rho(B, T) = \rho(B_c) f_\Delta[|B - B_c| / T^{1/2z\nu_\Delta}]. \quad (\text{S47})$$

### B. Without disorder

When  $\Delta_0 = \Delta_x = 0$ , and  $\gamma$  is a small quantity, there exist two fixed points, denoted as CFPs (i.e. Clean Fixed Point)

$$\text{CFP1: } (u_*, \beta_*) = (0, 0), \quad \text{CFP2: } (u_*, \beta_*) = \left(0, (1 + 1/\gamma)^2\right) \quad (\text{S48})$$

By linearizing the renormalization-group equations around CFP2, we obtain

$$\frac{d\delta u}{d\ell} = -2(\gamma + 1)\delta u, \quad (\text{S49})$$

$$\frac{d\delta\beta}{d\ell} = -2\delta\beta + \frac{2(\gamma + 1)^2}{\gamma^2}\delta u. \quad (\text{S50})$$

Both directions are irrelevant, and CFP2 is an stable and attractive fixed point. However, when  $\gamma \rightarrow 0$ ,  $\beta_* \rightarrow \infty$  for CFP2. The only physically achieved fixed point is CFP1. The linearized renormalization-group equations around this fixed point become

$$\frac{d\delta u}{d\ell} = 0, \quad (\text{S51})$$

$$\frac{d\delta\beta}{d\ell} = 2\delta\beta, \quad (\text{S52})$$

which indicates that  $\beta$  is a relevant variable near this fixed point, and it increases with  $\ell$  as  $e^{2\ell}$ . As a result, it gives rise to a correlation length exponent as  $\nu_\beta = 1/2$  [10]. It seems that  $u$  near this fixed point is marginal, but we remind that it is marginally irrelevant because once  $\beta$  departs from the Gaussian fixed point,  $u$  becomes irrelevant according to Eq. (S49).

### C. With forward-scattering disorder

For  $\Delta_f = 0$ , the fixed points are given by (FFPs for Forward-scattering-disorder Fixed points)

$$\text{FFP1: } (u_*, \beta_*) = (0, 0, 0), \quad \text{FFP2: } (u_*, \beta_*) = \left(0, (1 + 1/\gamma)^2, 0\right) \quad (\text{S53})$$

FFP1 is the clean and non-interacting fixed point, but is unstable. By linearizing the renormalization-group equations around FFP1, we obtain

$$\frac{d\delta u}{d\ell} = 0, \quad (\text{S54})$$

$$\frac{d\delta\beta}{d\ell} = 2\delta\beta, \quad (\text{S55})$$

$$\frac{d\delta\Delta_f}{d\ell} = \delta\Delta_f. \quad (\text{S56})$$

Near the fixed point, the electron-phonon coupling increases with  $\ell$  as  $e^{2\ell}$  the disorder increases with  $\ell$  as  $e^\ell$ . This fixed point is the multi-critical point for the CDW transition and Anderson transition. Considering that the  $\beta$  is the most relevant variable near this fixed point, the CDW transition is the first instability accompanied by the Anderson transition. As a result, the correlation length exponent is  $\nu_\beta = 1/2$  [10].

Around FFP2,

$$\frac{d\delta u}{d\ell} = -2(\gamma + 1)\delta u, \quad (\text{S57})$$

$$\frac{d\delta\beta}{d\ell} = -2\delta\beta + \frac{2(\gamma + 1)^2}{\gamma^2}\delta u - \frac{4(\gamma + 1)^2}{\gamma^2}\delta\Delta_f, \quad (\text{S58})$$

$$\frac{d\delta\Delta_f}{d\ell} = (1 - 4\gamma)\delta\Delta_f. \quad (\text{S59})$$

This is an attractive fixed point for  $\beta$  and represents the CDW phase with strong disorder scattering.

### D. With backscattering disorder

When  $\Delta_f = 0$ , the fixed points for the left couplings are given by (BFPs for Backscattering-disorder Fixed points)

$$\text{BFP2: } (u_*, \beta_*, \Delta_b^*) = (0, 0, 0); \quad \text{BFP2: } (u_*, \beta_*, \Delta_b^*) = \left(0, (1 + 1/\gamma)^2, 0\right); \quad (\text{S60})$$

$$\text{BFP3: } (u_*, \beta_*, \Delta_b^*) = (0, 0, 1/4); \quad \text{BFP4: } (u_*, \beta_*, \Delta_b^*) = (1/2, 0, 1/2) \quad (\text{S61})$$

By linearizing the renormalization-group equations around BFP1, we obtain

$$\frac{d\delta u}{d\ell} = 0, \quad (\text{S62})$$

$$\frac{d\delta\beta}{d\ell} = 2\delta\beta, \quad (\text{S63})$$

$$\frac{d\delta\Delta_b}{d\ell} = \delta\Delta_b. \quad (\text{S64})$$

Near the fixed point, the electron-phonon coupling increases with  $\ell$  as  $e^{2\ell}$  the disorder increases with  $\ell$  as  $e^\ell$ . Around BFP2, the linearized renormalization-group equations takes the form

$$\frac{d\delta u}{d\ell} = -2(\gamma + 1)\delta u, \quad (\text{S65})$$

$$\frac{d\delta\beta}{d\ell} = -2\delta\beta + \frac{2(\gamma + 1)^2}{\gamma^2}\delta u - \frac{4(\gamma + 1)^2}{\gamma^2}\delta\Delta_f, \quad (\text{S66})$$

$$\frac{d\delta\Delta_b}{d\ell} = (-1 - 4\gamma)\delta\Delta_b. \quad (\text{S67})$$

There is no relevant variable near this fixed point. This fixed point is stable for all three couplings. Linearizing the renormalization-group equations around BFP3 leads to

$$\frac{d\delta u}{d\ell} = -\frac{1}{2}\delta u, \quad (\text{S68})$$

$$\frac{d\delta\beta}{d\ell} = \delta\beta, \quad (\text{S69})$$

$$\frac{d\delta\Delta_b}{d\ell} = -\delta\Delta_b + \frac{1}{2}\delta u - \frac{\gamma^2(2\gamma + 1)\delta\beta}{2(\gamma + 1)^2}. \quad (\text{S70})$$

Only the electron-phonon coupling is unstable and gives rise to a correlation length exponent  $\nu_\beta = 1$ . This is the critical fixed point for electron-phonon induced CDW phase with stable and finite backscattering disorder coupling, and irrelevant electron-electron interactions. Around BFP4, the linearized renormalization-group equations are given by

$$\frac{d\delta u}{d\ell} = \delta u - \frac{\delta\beta\gamma^2}{\gamma + 1} - \delta\Delta_b, \quad (\text{S71})$$

$$\frac{d\delta\beta}{d\ell} = \delta\beta, \quad (\text{S72})$$

$$\frac{d\delta\Delta_b}{d\ell} = -2\delta\Delta_b + \delta u - \frac{\gamma^2(2\gamma + 1)\delta\beta}{(\gamma + 1)^2}. \quad (\text{S73})$$

Near the fixed point, both the electron-electron and electron-phonon couplings increase with  $\ell$  as  $e^\ell$ . This is a multi-critical point for the Perls transition and Wigner crystal transition.

- 
- [1] R. Y. Chen, Z. G. Chen, X.-Y. Song, J. A. Schneeloch, G. D. Gu, F. Wang, and N. L. Wang, *Phys. Rev. Lett.* **115**, 176404 (2015).  
[2] F. Tang, Y. Ren, P. Wang, R. Zhong, J. Schneeloch, S. A. Yang, K. Yang, P. A. Lee, G. Gu, Z. Qiao, and L. Zhang, *Nature* **569**, 537 (2019).  
[3] F. Qin, S. Li, Z. Z. Du, C. M. Wang, W. Zhang, D. Yu, H.-Z. Lu, and X. C. Xie, *Phys. Rev. Lett.* **125**, 206601 (2020).

- [4] Y. Jiang, Z. L. Dun, H. D. Zhou, Z. Lu, K.-W. Chen, S. Moon, T. Besara, T. M. Siegrist, R. E. Baumbach, D. Smirnov, and Z. Jiang, *Phys. Rev. B* **96**, 041101(R) (2017).
- [5] T. Giamarchi, *Quantum Physics in One Dimension* (Clarendon Press, 2003).
- [6] G. Grüner, *Density Waves in Solids* (Westview Press, 2000).
- [7] W. Kohn, *Phys. Rev. Lett.* **2**, 393 (1959).
- [8] S.-K. Jian and Z. Zhu, *Phys. Rev. Res.* **2**, 033414 (2020).
- [9] R. Shankar, *Rev. Mod. Phys.* **66**, 129 (1994).
- [10] P. Goswami and S. Chakravarty, *Phys. Rev. Lett.* **107**, 196803 (2011).
- [11] H.-Z. Lu, S.-B. Zhang, and S.-Q. Shen, *Phys. Rev. B* **92**, 045203 (2015).
- [12] A. A. Abrikosov, *Phys. Rev. B* **58**, 2788 (1998).
- [13] J. Zhu, T. Feng, S. Mills, P. Wang, X. Wu, L. Zhang, S. T. Pantelides, X. Du, and X. Wang, *ACS Applied Materials & Interfaces* **10**, 40740 (2018), <https://doi.org/10.1021/acsami.8b12504>.
- [14] M. Imada, A. Fujimori, and Y. Tokura, *Rev. Mod. Phys.* **70**, 1039 (1998).
- [15] S. L. Sondhi, S. M. Girvin, J. P. Carini, and D. Shahar, *Rev. Mod. Phys.* **69**, 315 (1997).
- [16] M. P. A. Fisher, *Phys. Rev. Lett.* **65**, 923 (1990).
